# Supplementary material for: Simple CHT: A New Derivation of the Weakest Failure Detector for Consensus
Source: arXiv:1310.1761 source file (2014-09-18)
Supplement: Supplementary file 2 [file supp-pdf.tex]

%D \module
%D   [       file=supp-pdf,
%D        version=2003.01.20,
%D          title=\CONTEXT\ Support Macros,
%D       subtitle=\METAPOST\ to \PDF\ conversion,
%D         author=Hans Hagen,
%D           date=\currentdate,
%D      copyright={PRAGMA / Hans Hagen \& Ton Otten}]
%C
%C This module is part of the \CONTEXT\ macro||package and is
%C therefore copyrighted by \PRAGMA. See mreadme.pdf for 
%C details. 

% This method is not that accurate with small files that use
% penshapes. I tried several methods but so far I could not
% come up with a better alternative. \TEX's real calculation
% options are simply to simple. Using \ETEX's expression
% mechanism does not lead to better results. 

% beware, we cannot use \zeropoint here since it may be 
% defined in the range \dimen 0 - 20 which we happen to use 
% as scratch registers ; inside context we may consider 
% using dedicated registers 

%D These macros are written as generic as possible. Some
%D general support macro's are loaded from a small module
%D especially made for non \CONTEXT\ use. In this module I
%D use a matrix transformation macro written by Tanmoy
%D Bhattacharya. Thanks to extensive testing by Sebastian
%D Ratz I was able to complete this module within reasonable
%D time. This module has support for \METAPOST\ extensions 
%D built in.

%D First we take care of non||\CONTEXT\ use:

\ifx \undefined \writestatus          \input supp-mis.tex \relax \fi
\ifx \undefined \convertMPtoPDF \else \expandafter \endinput     \fi 
\ifx \undefined \StartLatexHack \else \StartLatexHack            \fi 

%D This module handles some \PDF\ conversion and insertions
%D topics. By default, the macros use the \PDFTEX\ primitive
%D \type{\pdfliteral} when available. 

\writestatus{loading}{Context Support Macros / PDF}

\unprotect

\ifx\PDFcode\undefined
  \ifx\pdfliteral\undefined
    \def\PDFcode#1{\special{PDF: #1}}
  \else
    \let\PDFcode\pdfliteral
  \fi
\fi

%D \macros 
%D   {pdfimage,pdfimages,pdfclippedimage}
%D
%D Starting with pdftex version 14, images are included more
%D natural to the form embedding. This enables alternative 
%D images to be embedded. 
%D
%D \starttypen
%D \pdfimage  <optional dimensions> {file}
%D \pdfimages <optional dimensions> {high res file} {low res file}
%D \stoptypen
%D
%D The first one replaces the pre||version||14 original, 
%D while the latter provides alternative images. 
%D 
%D The next macro is dedicated to Maarten Gelderman, who 
%D needed to paste prepared \PDF\ pages into conference 
%D proceedings.
%D 
%D \starttypen
%D \pdfclippedimage <optional dimensions> {file} {l} {r} {t} {b} 
%D \stoptypen

\ifx\pdftexversion\undefined % no \m!systems for the sake of latex
  \writestatus{systems}{Why not use pdf(e)TeX binaries?}
  \protect 
  \expandafter\endinput 
\fi 

\ifnum\pdftexversion>13 

  \def\pdfimage#1#%
    {\dopdfimage{#1}}

  \def\dopdfimage#1#2%
    {\immediate\pdfximage#1{#2}%
     \pdfrefximage\pdflastximage}

  \def\pdfimages#1#%
    {\dopdfimages{#1}}

  \def\dopdfimages#1#2#3%
    {\immediate\pdfximage#1{#2}%
     \immediate\pdfobj
       {[ << /Image \the\pdflastximage\space0 R 
             /DefaultForPrinting true >> ]}%
     \immediate\pdfximage#1 
       attr {/Alternates \the\pdflastobj\space0 R}{#3}%
     \pdfrefximage\pdflastximage}

  \def\pdfclippedimage#1#% specs {file}{left}{right}{top}{bottom} 
    {\dopdfclippedimage{#1}}

  \def\dopdfclippedimage#1#2#3#4#5#6% 
    {\bgroup
     \pdfximage#1{#2}%
     \setbox\scratchbox\hbox
       {\pdfrefximage\pdflastximage}%
     \hsize\wd\scratchbox
     \advance\hsize -#3 
     \advance\hsize -#4 
     \vsize\ht\scratchbox
     \advance\vsize -#5 
     \advance\vsize -#6 
     \setbox\scratchbox\vbox to \vsize
       {\vskip-#5\hbox to \hsize{\hskip-#3\box\scratchbox\hss}}%
     \pdfxform\scratchbox
     \pdfrefxform\pdflastxform
     \egroup}

%D If you want to save a few hash entries, you may prefer the 
%D less readable alternatives, like:  
%D  
%D \starttypen 
%D \def\pdfimage#1#% This one is less readable but needs no additional
%D   {\bgroup      % hash entry for the second stage macro.   
%D    \def\pdfimage##1%
%D      {\immediate\pdfximage##1{#2}%
%D       \pdfrefximage\pdflastximage\egroup}}
%D \stoptypen

%D For old times sake: (will be removed some day)

  \let\pdfform    =\pdfxform
  \let\pdflastform=\pdflastxform
  \let\pdfrefform =\pdfrefxform

\fi

%D \macros
%D   {convertPDFtoPDF}
%D
%D \PDFTEX\ supports verbatim inclusion of \PDF\ code. The
%D following macro takes care of inserting externally defined
%D illustrations in \PDF\ format. According to a suggestion
%D Tanmoy Bhattacharya posted to the \PDFTEX\ mailing list, we
%D first skip lines until \type{stream} is reached and then
%D copy lines until \type{endstream} is encountered. This
%D scheme only works with vectorized graphics in which no
%D indirect references to objects are used. Bitmaps also don't
%D work. Interpreting their specifications is beyond the
%D current implementation.
%D
%D \starttypen
%D \convertPDFtoPDF
%D   {filename}
%D   {x scale} {y scale}
%D   {x offset } {y offset}
%D   {width} {height}
%D \stoptypen
%D
%D When the scales are set to~1, the last last four values
%D are the same as the bounding box, e.g.
%D
%D \starttypen
%D \convertPDFtoPDF{mp-pra-1.pdf} {1} {1}{-1bp}{-1bp}{398bp}{398bp}
%D \convertPDFtoPDF{mp-pra-1.pdf}{.5}{.5} {0bp} {0bp}{199bp}{199bp}
%D \stoptypen
%D
%D Keep in mind, that this kind of copying only works for
%D pure and valid pdf code (without fonts).

%D The scanning and copying is straightforward and quite fast.
%D To speed up things we use two constants.

\def\@@PDFstream@@    {stream}
\def\@@PDFendstream@@ {endstream}

%D \macros
%D   {PDFmediaboxprefered}
%D
%D If needed, the macros can scan for the mediabox that
%D specifies the dimensions and offsets of the graphic. When
%D we say:
%D
%D \starttypen
%D \PDFmediaboxpreferedtrue
%D \stoptypen
%D
%D the mediabox present in the file superseded the user
%D specified, already scaled and calculated offset and
%D dimensions. Beware: the user supplied values are not the
%D bounding box ones!

% this will become obsolete 

\newif\ifPDFmediaboxprefered

\def\setPDFboundingbox#1#2#3#4#5#6%
  {\dimen0=#1\dimen0=#5\dimen0
   \ScaledPointsToBigPoints{\number\dimen0}\PDFxoffset
   \dimen0=#3\dimen0=#5\dimen0
   \xdef\PDFwidth{\the\dimen0}%
   \dimen0=#2\dimen0=#6\dimen0
   \ScaledPointsToBigPoints{\number\dimen0}\PDFyoffset
   \dimen0=#4\dimen0=#6\dimen0
   \xdef\PDFheight{\the\dimen0}%
   \global\let\PDFxoffset\PDFxoffset
   \global\let\PDFyoffset\PDFyoffset}

\def\setPDFmediabox#1[#2 #3 #4 #5]#6\done%
  {\dimen2=#2bp\dimen2=-\dimen2
   \dimen4=#3bp\dimen4=-\dimen4
   \dimen6=#4bp\advance\dimen6 \dimen2
   \dimen8=#5bp\advance\dimen8 \dimen4
   \setPDFboundingbox{\dimen2}{\dimen4}{\dimen6}{\dimen8}\PDFxscale\PDFyscale}

\def\checkPDFmediabox#1/MediaBox#2#3\done%
  {\ifx#2\relax \else
     \message{mediabox}%
     \setPDFmediabox#2#3\done
   \fi}

%D We use the general macro \type{\doprocessfile} and feed this
%D with a line handling macro that changes it's behavior when
%D the stream operators are encountered.

\def\handlePDFline%
  {\ifx\@@PDFstream@@\fileline
     \let\doprocessPDFline\copyPDFobject
     \startPDFtoPDF
   \else\ifPDFmediaboxprefered
     \expandafter\checkPDFmediabox\fileline/MediaBox\relax\done
   \fi\fi}

\def\copyPDFobject%
  {\ifx\@@PDFendstream@@\fileline
     \ifPDFmediaboxprefered
       \let\doprocessPDFline\findPDFmediabox
     \else
       \let\doprocessPDFline\relax
     \fi
   \else
     \advance\scratchcounter 1
     \PDFcode{\fileline}%
   \fi}

\def\findPDFmediabox%
  {\expandafter\checkPDFmediabox\fileline/MediaBox\relax\done}

%D The main conversion macro wraps the \PDF\ codes in a box
%D that is output as an object. The graphics are embedded
%D in~\type{q} and~\type{Q} and are scaled and positioned using
%D one transform call (\type{cm}). This saves some additional
%D scaling.

%D \starttypen
%D \def\startPDFtoPDF%
%D   {\setbox0=\vbox\bgroup
%D      \message{[PDF to PDF \PDFfilename}%
%D      \forgetall
%D      \scratchcounter=0
%D      \let\stopPDFtoPDF=\dostopPDFtoPDF}
%D 
%D \def\dostopPDFtoPDF%
%D   {\ifnum\scratchcounter<0 \scratchcounter=1 \fi
%D    \message{(\the\scratchcounter\space lines)]}%
%D    \egroup
%D    \wd0=\PDFwidth
%D    \vbox to \PDFheight
%D      {\forgetall
%D       \vfill
%D       \PDFcode{q}%
%D       \PDFcode{1 0 0 1 \PDFxoffset\space \PDFyoffset\space cm}%
%D       \PDFcode{\PDFxscale\space 0 0 \PDFyscale\space 0 0 cm}%
%D       \box0
%D       \PDFcode{Q}}}
%D 
%D \def\stopPDFtoPDF%
%D    {\message{[PDF to PDF \PDFfilename\space not found]}}
%D 
%D \def\convertPDFtoPDF#1#2#3#4#5#6#7%
%D   {\bgroup
%D    \def\PDFfilename{#1}%
%D    \def\PDFxscale  {#2}%
%D    \def\PDFyscale  {#3}%
%D    \setPDFboundingbox{#4}{#5}{#6}{#7}{1}{1}%
%D    \uncatcodespecials
%D    \endlinechar=-1
%D    \let\doprocessPDFline=\handlePDFline
%D    \doprocessfile\scratchread\PDFfilename\doprocessPDFline
%D    \stopPDFtoPDF
%D    \egroup}

\def\convertPDFtoPDF#1#2#3#4#5#6#7%
  {\message{[PDF to PDF use \string\PDFcode instead]}%
   \vbox{use the direct method instead}}

%D \macros 
%D   {dogetPDFmediabox}
%D
%D The next macro can be used to find the mediabox of a \PDF\
%D illustration. 
%D
%D \starttypen
%D \dogetPDFmediabox
%D   {filename}
%D   {new dimen}{new dimen}{new dimen}{new dimen} 
%D \stoptypen
%D
%D Beware of dimen clashes: this macro uses the 5~default  
%D scratch registers! When no file or mediabox is found, the 
%D dimensions are zeroed. 

\def\dogetPDFmediabox#1#2#3#4#5%
  {\bgroup
   \def\PDFxscale{1}%
   \def\PDFyscale{1}%
   \uncatcodespecials
   \endlinechar=-1
   \def\checkPDFtypepage##1/Type /Page##2##3\done%
     {\ifx##2\relax 
      \else\if##2s% accept /Page and /Pages 
        \let\doprocessPDFline\findPDFmediabox
      \else
        \let\doprocessPDFline\findPDFmediabox
      \fi\fi}%
   \def\findPDFtypepage%
     {\expandafter\checkPDFtypepage\fileline/Type /Page\relax\done}%
   \def\checkPDFmediabox##1/MediaBox##2##3\done%
     {\ifx##2\relax \else
        \setPDFmediabox##2##3\done
        \fileprocessedtrue
      \fi}%
   \def\findPDFmediabox%
     {\expandafter\checkPDFmediabox\fileline/MediaBox\relax\done}%
   \let\doprocessPDFline\findPDFtypepage
   \doprocessfile\scratchread{#1}\doprocessPDFline
   \egroup
   \ifx\PDFxoffset\undefined
     #2=\!!zeropoint   #3=\!!zeropoint   #4=\!!zeropoint #5=\!!zeropoint
   \else
     #2=\PDFxoffset bp #3=\PDFyoffset bp #4=\PDFwidth    #5=\PDFheight
   \fi}

%D \macros
%D   {convertMPtoPDF}
%D
%D The next set of macros implements \METAPOST\ to \PDF\
%D conversion. Because we want to test as fast as possible, we
%D first define the \POSTSCRIPT\ operators that \METAPOST\
%D uses. We don't define irrelevant ones, because these are
%D skipped anyway.

%D The converter can be made a bit faster by replacing the 
%D two test macros (the ones with the many \type {\if's}) by 
%D a call to named branch macros (something \typ {\getvalue 
%D {xPSmoveto}}. For everyday documents with relatively 
%D small graphics the gain in speed can be neglected.  

\def \PScurveto          {curveto}
\def \PSlineto           {lineto}
\def \PSmoveto           {moveto}
\def \PSshowpage         {showpage}
\def \PSnewpath          {newpath}
\def \PSfshow            {fshow}
\def \PSclosepath        {closepath}
\def \PSfill             {fill}
\def \PSstroke           {stroke}
\def \PSclip             {clip}
\def \PSrlineto          {rlineto}
\def \PSsetlinejoin      {setlinejoin}
\def \PSsetlinecap       {setlinecap}
\def \PSsetmiterlimit    {setmiterlimit}
\def \PSsetgray          {setgray}
\def \PSsetrgbcolor      {setrgbcolor}
\def \PSsetcmykcolor     {setcmykcolor}
\def \PSsetdash          {setdash}
\def \PSgsave            {gsave}
\def \PSgrestore         {grestore}
\def \PStranslate        {translate}
\def \PSscale            {scale}
\def \PSconcat           {concat}
\def \PSdtransform       {dtransform}

\def \PSnfont            {nfont}    % was needed for TUG98 proceedings 
\def \PSspecial          {special}  % extensions to MetaPost
 
\def \PSBoundingBox      {BoundingBox:}
\def \PSHiResBoundingBox {HiResBoundingBox:}
\def \PSExactBoundingBox {ExactBoundingBox:}
\def \PSMetaPostSpecial  {MetaPostSpecial:}
\def \PSMetaPostSpecials {MetaPostSpecials:}
\def \PSPage             {Page:}

%D By the way, the \type {setcmykcolor} operator is not
%D output by \METAPOST\ but can result from converting the
%D \kap{RGB} color specifications, as implemented in
%D \type{supp-mps}.

%D In \POSTSCRIPT\ arguments precede the operators. Due to the
%D fact that in some translations we need access to those
%D arguments, and also because sometimes we have to skip them,
%D we stack them up. The stack is one||dimensional for non path
%D operators and two||dimensional for operators inside a path.
%D This is because we have to save the whole path for
%D (optional) postprocessing. Values are pushed onto the stack
%D by:
%D
%D \starttypen
%D \setMPargument {value}
%D \stoptypen
%D
%D They can be retrieved by the short named macros:
%D
%D \starttypen
%D \gMPa {number}
%D \gMPs {number}
%D \stoptypen
%D
%D When scanning a path specification, we also save the
%D operator, using
%D
%D \starttypen
%D \setMPkeyword {n}
%D \stoptypen
%D
%D The path drawing operators are coded for speed: \type{clip},
%D \type{stroke}, \type{fill} and \type{fillstroke} become
%D 1, 2, 3 and~4.
%D
%D When processing the path this code can be retrieved
%D using
%D
%D \starttypen
%D \getMPkeyword{n}
%D \stoptypen
%D
%D When setting an argument, the exact position on the stack
%D depends on the current value of the \COUNTERS\
%D \type{\nofMPsegments} and \type{\nofMParguments}.

\newcount\nofMPsegments
\newcount\nofMParguments

%D These variables hold the coordinates. The argument part of
%D the stack is reset by:
%D
%D \starttypen
%D \resetMPstack
%D \stoptypen
%D
%D We use the prefix \type{@@MP} to keep the stack from
%D conflicting with existing macros. To speed up things a bit
%D more, we use the constant \type{\@@MP}.

\def\@@MP{@@MP}

\def\setMPargument% #1%
  {\advance\nofMParguments 1
   \expandafter\def
     \csname\@@MP\the\nofMPsegments\the\nofMParguments\endcsname} % {#1}

\def\letMPargument
  {\advance\nofMParguments 1
   \expandafter\let
     \csname\@@MP\the\nofMPsegments\the\nofMParguments\endcsname}

\def\setMPsequence#1 %
  {\advance\nofMParguments 1
   \expandafter\def
     \csname\@@MP\the\nofMPsegments\the\nofMParguments\endcsname{#1}%
   \handleMPsequence}

\def\gMPa#1%
  {\csname\@@MP0\number#1\endcsname}

\def\gMPs#1%
  {\csname\@@MP\the\nofMPsegments\number#1\endcsname}

\def\dogMPa#1%
  {\@EAEAEA\do\csname\@@MP0\number#1\endcsname}

\def\setMPkeyword#1 % 
  {\expandafter\def\csname\@@MP\the\nofMPsegments0\endcsname{#1}%
   \advance\nofMPsegments1
   \nofMParguments0 }

\def\getMPkeyword#1%
  {\csname\@@MP#10\endcsname}

%D When we reset the stack, we can assume that all further
%D comment is to be ignored and handled in strings.
%D By redefining the reset macro after the first call, we
%D save some run time. Only use this macro after all 
%D comments are processed and use the simple alternative 
%D when dealing with comments. 

\def\doresetMPstack%
  {\nofMParguments0 }

\def\resetMPstack%
  {\catcode`\%=\@@active
   \let\handleMPgraphic\handleMPendgraphic
   \let\resetMPstack\doresetMPstack
   \resetMPstack}

%D The arguments are saved with the preceding command
%D \type{\do}. By default this command expands to nothing, but
%D when we deal with strings it's used to strip off the
%D \type{(} and \type{)}.
%D
%D Strings are kind of tricky, because characters can be
%D passed verbatim \type{(hello)}, by octal number
%D \type{(\005)} or as command \type{(\()}. We therefore
%D cannot simply ignore \type{(} and \type{)}, the way we do
%D with \type{[} and \type{]}. Another complication is that
%D strings may contain characters that normally have a
%D special meaning in \TEX, like \type{$} and \type{{}}.
%D
%D A previous solution made \type{\} an active character and
%D let it look ahead for a number or characters. We had to
%D abandon this scheme because of the need for verbatim
%D support. The next solution involved some \CATCODE\
%D trickery but works well.

\def\octalMPcharacter#1#2#3%
  {\char'#1#2#3\relax}

\bgroup
\catcode`\|=\@@comment
\catcode`\%=\@@active
\catcode`\[=\@@active
\catcode`\]=\@@active
\catcode`\{=\@@active
\catcode`\}=\@@active
\catcode`B=\@@begingroup
\catcode`E=\@@endgroup
\gdef\ignoreMPspecials|
  B\def%BE|
   \def[BE|
   \def]BE|
   \def{BE|
   \def}BEE
\gdef\obeyMPspecials|
  B\def%B\char 37\relax E|
   \def[B\char 91\relax E|
   \def]B\char 93\relax E|
   \def{B\char123\relax E|
   \def}B\char125\relax EE
\gdef\setMPspecials|
  B\setnaturalcatcodes
   \catcode`\\=\@@escape
   \catcode`\%=\@@active
   \catcode`\[=\@@active
   \catcode`\]=\@@active
   \catcode`\{=\@@active
   \catcode`\}=\@@active
   \def\(B\char40\relax     E|
   \def\)B\char41\relax     E|
   \def\\B\char92\relax     E|
   \def\0B\octalMPcharacter0E|
   \def\1B\octalMPcharacter1E|
   \def\2B\octalMPcharacter2E|
   \def\3B\octalMPcharacter3E|
   \def\4B\octalMPcharacter4E|
   \def\5B\octalMPcharacter5E|
   \def\6B\octalMPcharacter6E|
   \def\7B\octalMPcharacter7E|
   \def\8B\octalMPcharacter8E|
   \def\9B\octalMPcharacter9EE
\egroup

%D We use the comment symbol as a sort of trigger:

\bgroup
\catcode`\%=\@@active
\gdef\startMPscanning{\let%=\startMPconversion}
\egroup

%D In earlier versions we used the sequence
%D
%D \starttypen
%D \expandafter\handleMPsequence\input filename\relax
%D \stoptypen
%D
%D Persistent problems in \LATEX\ however forced us to use a
%D different scheme. Every \POSTSCRIPT\ file starts with a
%D \type{%}, so we temporary make this an active character
%D that starts the scanning and redefines itself. (The problem
%D originates in the redefinition by \LATEX\ of the
%D \type{\input} primitive.)

\def\startMPconversion%
  {\catcode`\%=\@@ignore
   \ignoreMPspecials
   \handleMPsequence}

%D Here comes the main loop. Most arguments are numbers. This
%D means that they can be recognized by their \type{\lccode}.
%D This method saves a lot of processing time. We could
%D speed up the conversion by handling the \type{path}
%D seperately.

\def\@EAEAEA{\expandafter\expandafter\expandafter} % to be sure 

\def\dohandleMPsequence#1%
  {\ifdone
     \ifcase\lccode`#1\relax 
       \@EAEAEA\dohandleMPsequenceA
     \else
       \@EAEAEA\dohandleMPsequenceB
     \fi
   \else
     \@EA\dohandleMPsequenceC
   \fi#1} 

%\def\dohandleMPsequenceA#1 %
%  {\setMPargument{#1}%
%   \handleMPsequence}
 
\let\dohandleMPsequenceA\setMPsequence

\def\dohandleMPsequenceB#1 %
  {\edef\somestring{#1}%
   \ifx\somestring\PSmoveto
     \edef\lastMPmoveX{\gMPa1}%
     \edef\lastMPmoveY{\gMPa2}%
     \PDFcode{\!MPgMPa1 \!MPgMPa2 m}%
     \resetMPstack
   \else\ifx\somestring\PSnewpath
     \let\handleMPsequence\handleMPpath
   \else\ifx\somestring\PSgsave
     \PDFcode{q}%
     \resetMPstack
   \else\ifx\somestring\PSgrestore
     \PDFcode{Q}%
     \resetMPstack
   \else\ifx\somestring\PSdtransform  % == setlinewidth
     \let\handleMPsequence\handleMPdtransform
   \else\ifx\somestring\PSconcat
     \PDFcode{\gMPa1 \gMPa2 \gMPa3 \gMPa4 \gMPa5 \gMPa6 cm}%
     \resetMPstack
   \else\ifx\somestring\PSsetrgbcolor
     \handleMPrgbcolor
     \resetMPstack
   \else\ifx\somestring\PSsetcmykcolor
     \handleMPcmykcolor
     \resetMPstack
   \else\ifx\somestring\PSsetgray
     \handleMPgraycolor
     \resetMPstack
   \else\ifx\somestring\PStranslate
     \PDFcode{1 0 0 1 \gMPa1 \gMPa2 cm}%
     \resetMPstack
   \else\ifx\somestring\PSsetdash
     \handleMPsetdash
     \resetMPstack
   \else\ifx\somestring\PSsetlinejoin
     \PDFcode{\gMPa1 j}%
     \resetMPstack
   \else\ifx\somestring\PSsetmiterlimit
     \PDFcode{\gMPa1 M}%
     \resetMPstack
   \else\ifx\somestring\PSfshow
     \PDFcode{n}% 
     \handleMPfshow
     \resetMPstack
   \else\ifx\somestring\PSsetlinecap
     \PDFcode{\gMPa1 J}%
     \resetMPstack
   \else\ifx\somestring\PSrlineto
     \PDFcode{\!MP\lastMPmoveX\space\!MP\lastMPmoveY\space l S}%
     \resetMPstack
   \else\ifx\somestring\PSscale
     \PDFcode{\gMPa1 0 0 \gMPa2 0 0 cm}%
     \resetMPstack
   \else\ifx\somestring\PSspecial
     \handleMPspecialcommand
     \resetMPstack
   \else
     \handleMPgraphic% {#1}%
   \fi\fi\fi\fi\fi\fi\fi\fi\fi\fi\fi\fi\fi\fi\fi\fi\fi\fi
   \handleMPsequence}

\def\dohandleMPsequenceC#1 %
  {\edef\somestring{#1}%
   \handleMPgraphic % {#1}%
   \handleMPsequence}

%D Since colors are not sensitive to transformations, they 
%D are sometimes used for signaling. Therefore, we handle them 
%D separately. The next macro can be redefined if needed. 

\def\handleMPrgbcolor
  {\PDFcode{\!MPgMPa1 \!MPgMPa2 \!MPgMPa3 rg 
            \!MPgMPa1 \!MPgMPa2 \!MPgMPa3 RG}}

\def\handleMPcmykcolor
  {\PDFcode{\!MPgMPa1 \!MPgMPa2 \!MPgMPa3 \!MPgMPa4 k 
            \!MPgMPa1 \!MPgMPa2 \!MPgMPa3 \!MPgMPa4 K}}

\def\handleMPgraycolor
  {\PDFcode{\!MPgMPa1 g 
            \!MPgMPa1 G}}

\def\handleMPspotcolor
  {\PDFcode{0 g 
            0 G}}

%D Beginning and ending the graphics is taken care of by the
%D macro \type{\handleMPgraphic}, which is redefined when
%D the first graphics operator is met.

\def\handleMPendgraphic % #1%
  {\ifx\somestring\PSshowpage
     \let\handleMPsequence\finishMPgraphic
   \else
     \letMPargument\somestring % {#1}%
   \fi}

\def\handleMPbegingraphic % #1%
  {\ifx\somestring\PSBoundingBox
     \def\handleMPsequence{\handleMPboundingbox1}%
   \else\ifx\somestring\PSHiResBoundingBox
     \def\handleMPsequence{\handleMPboundingbox2}%
   \else\ifx\somestring\PSExactBoundingBox
     \def\handleMPsequence{\handleMPboundingbox3}%
   \else\ifx\somestring\PSshowpage
     \let\handleMPsequence\finishMPgraphic
   \else\ifx\somestring\PSPage
     \let\handleMPsequence\handleMPpage
   \else\ifx\somestring\PSMetaPostSpecials
     \let\handleMPsequence\handleMPspecialscomment
   \else\ifx\somestring\PSMetaPostSpecial
     \let\handleMPsequence\handleMPspecialcomment
   \else
     \letMPargument\somestring % {#1}% 
   \fi\fi\fi\fi\fi\fi\fi}

\let\handleMPgraphic=\handleMPbegingraphic

%D We check for three kind of bounding boxes: the normal one
%D and two high precision ones:
%D
%D \starttypen
%D BoundingBox: llx lly ucx ucy
%D HiResBoundingBox: llx lly ucx ucy
%D ExactBoundingBox: llx lly ucx ucy
%D \stoptypen
%D
%D The original as well as the recalculated dimensions are 
%D saved for later use.

\newif\ifskipemptyMPgraphic \skipemptyMPgraphicfalse

\chardef\currentMPboundingbox=0

\def\handleMPboundingbox#1#2 #3 #4 #5
  {\ifnum#1>\currentMPboundingbox
     \xdef\MPllx{#2}\xdef\MPlly{#3}%
     \xdef\MPurx{#4}\xdef\MPury{#5}%
     \dimen0=#2pt\dimen0=-\MPxscale\dimen0
     \dimen2=#3pt\dimen2=-\MPyscale\dimen2
     \xdef\MPxoffset{\withoutpt{\the\dimen0}}%
     \xdef\MPyoffset{\withoutpt{\the\dimen2}}%
     \dimen0=#2bp\dimen0=-\dimen0
     \dimen2=#3bp\dimen2=-\dimen2
     \advance\dimen0 #4bp
     \dimen0=\MPxscale\dimen0
     \xdef\MPwidth{\the\dimen0}%
     \advance\dimen2 #5bp
     \xdef\MPyshift{\the\dimen2}% unscaled 
     \dimen2=\MPyscale\dimen2
     \xdef\MPheight{\the\dimen2}%
     \chardef\currentMPboundingbox=#1\relax
   \fi
   \doresetMPstack
   \let\handleMPsequence\dohandleMPsequence
   \let\next\handleMPsequence
   \ifskipemptyMPgraphic
     \ifdim\MPheight=\!!zeropoint\relax\ifdim\MPwidth=\!!zeropoint\relax
      \def\next{\endinput\finishMPgraphic}%
     \fi\fi
   \fi
   \next}

%D Unless defined otherwise, we simply ignore specialcomments. 

\def\handleMPspecialcomment%
  {\doresetMPstack
   \let\handleMPsequence\dohandleMPsequence
   \handleMPsequence}

\let\handleMPspecialscomment\handleMPspecialcomment

%D We use the \type{page} comment as a signal that
%D stackbuilding can be started.

\def\handleMPpage #1 #2
  {\doresetMPstack
   \donetrue
   \let\handleMPsequence\dohandleMPsequence
   \handleMPsequence}

%D The same applies to the special extensions. 

\def\handleMPspecialcommand 
  {\doresetMPstack
   \let\handleMPsequence\dohandleMPsequence
   \handleMPsequence}

%D \METAPOST\ draws its dots by moving to a location and
%D invoking \type{0 0 rlineto}. This operator is not
%D available in \PDF. Our solution is straightforward: we draw
%D a line from $(current\_x, current\_y)$ to itself. This
%D means that the arguments of the preceding \type{moveto} have
%D to be saved.

\def\lastMPmoveX{0}
\def\lastMPmoveY{0}

%D These saved coordinates are also used when we handle the
%D texts. Text handling proved to be a bit of a nuisance, but
%D finally I saw the light. It proved that we also had to
%D take care of \type{(split arguments)}.

\def\setMPfshowfont#1#2%
  {\font\temp=#1\space at #2\relax\temp}

\let\MPfshowcommand\empty

\def\handleMPfshow
  {\bgroup
   \setbox\scratchbox\hbox
     {\obeyMPspecials
      \edef\size{\gMPa\nofMParguments}%
      \ifx\size\PSnfont % round font size (to pt) 
        \advance\nofMParguments -1
        \expandafter\scratchdimen\gMPa\nofMParguments pt\relax
        \ifdim\scratchdimen<1pt
          \def\size{1pt}%
        \else
          \advance\scratchdimen .5pt 
          \def\size##1.##2\relax{\def\size{##1pt}}% 
          \expandafter\size\the\scratchdimen\relax
        \fi
      \else
        \edef\size{\size bp}%
      \fi
      \advance\nofMParguments -1
     %\font\temp=\gMPa\nofMParguments\space at \size
      \let\temp\relax % to be sure 
      \setMPfshowfont{\gMPa\nofMParguments}\size
      \advance\nofMParguments -1
      \temp
      \MPfshowcommand
        {\ifnum\nofMParguments=1
           \def\do(##1){##1}%
           \dogMPa1%
         \else
           % we need to catch ( a ) (a a a) (\123 \123 \123) etc 
           \scratchcounter=1
           \def\dodo##1% Andreas Fieger's bug: (\304...) 
             {\edef\!!stringa{##1\empty\empty}% and another one: ( 11) -> \ifx 11 
              \ifx\!!stringa\MPspacechar\MPspacechar\else\expandafter##1\fi}%
           \def\do(##1{\dodo{##1}}%
           \dogMPa\scratchcounter\MPspacechar 
           \let\do\relax
           \loop
             \advance\scratchcounter 1
             \ifnum\scratchcounter<\nofMParguments\relax
               \gMPa\scratchcounter\MPspacechar
           \repeat
           \def\do##1){\dodo{##1}}%
           \dogMPa\scratchcounter
         \fi
         \unskip}}%
  % 
  % this fails in latest pdftex's
  %
  % \dimen0=\lastMPmoveY bp
  % \advance\dimen0 by \ht0
  % \ScaledPointsToBigPoints{\number\dimen0}\lastMPmoveY
  % \PDFcode{n q 1 0 0 1 \lastMPmoveX\space\lastMPmoveY\space cm}%
  % \dimen0=\ht0
  % \advance\dimen0 by \dp0
  % \box0
  % \vskip-\dimen0
  % \PDFcode{Q}%
  % \egroup}
  %
   \setbox\scratchbox\hbox
     {\hskip\lastMPmoveX bp\raise\lastMPmoveY bp\box\scratchbox}%
   \ht\scratchbox\!!zeropoint
   \dp\scratchbox\!!zeropoint
   \wd\scratchbox\!!zeropoint
   \box\scratchbox
   \egroup}

%D You could consider the following definition to be the most
%D natural one. 

% \def\MPspacechar{\space} % normal case 

\def\MPspacechar{\char32\relax} % old solution does not work with math

%D However, the following implementation is more robust, since
%D some fonts have funny visible spaces in the space slot. This
%D gives a mismatch between the space that \METAPOST\ took into
%D account and the \citeer {natural} space. This only happens in
%D labels, since \type {btex}||\type {etex} thingies don't have
%D spaces. This phenomena showed up when preparing the
%D \METAFUN\ manual, where Palatino fonts are used. We can 
%D safely assume that \METAPOST\ considers \type {\char32} to 
%D be the space.  

\def\MPspacechar{\setbox\scratchbox\hbox{\char32}\kern\wd\scratchbox}

%D Well, this does not work with math fonts, so: 

\def\MPspacechar{\char32\relax}

%D Most operators are just converted and keep their
%D arguments. Dashes however need a bit different treatment,
%D otherwise \PDF\ viewers complain loudly. Another
%D complication is that one argument comes after the \type{]}.
%D When reading the data, we simply ignore the array boundary
%D characters. We save ourselves some redundant newlines and
%D at the same time keep the output readable by packing the
%D literals.

\def\handleMPsetdash%
  {\bgroup
   \def\somestring{[}%
   \scratchcounter1
   \loop
     \ifnum\scratchcounter<\nofMParguments
       \edef\somestring{\somestring\space\gMPa\scratchcounter}%
       \advance\scratchcounter 1
   \repeat
   \edef\somestring{\somestring]\gMPa\scratchcounter\space d}%
   \PDFcode{\somestring}%
   \egroup}

%D The \type{setlinewidth} commands looks a bit complicated. There are
%D two alternatives, that result in a similar look in both 
%D $x$- and $y$-dorection. As John Hobby says:
%D
%D \startsmaller \switchtobodyfont[ss]
%D \starttypen
%D x 0 dtransform exch truncate exch idtransform pop setlinewidth
%D 0 y dtransform truncate idtransform setlinewidth pop
%D \stoptypen
%D
%D These are just fancy versions of \type{x setlinewidth} and
%D \type{y setlinewidth}. The \type{x 0 ...} form is used if
%D the path is {\em primarily vertical}. It rounds the width
%D so that vertical lines come out an integer number of pixels
%D wide in device space. The \type{0 y ...} form does the same
%D for paths that are {\em primarily horizontal}. The reason
%D why I did this is Knuth insists on getting exactly the
%D widths \TEX\ intends for the horizontal and vertical rules
%D in \type{btex...etex} output. (Note that PostScript scan
%D conversion rules cause a horizontal or vertical line of
%D integer width $n$ in device space to come out $n+1$ pixels
%D wide, regardless of the phase relative to the pixel grid.)
%D \stopsmaller
%D
%D The common operator in these sequences is \type{dtransform},
%D so we can use this one to trigger setting the linewidth.

\def\handleMPdtransform%
  {\ifdim\gMPa1pt>\!!zeropoint
     \PDFcode{\gMPa1 w}%
     \def\next##1 ##2 ##3 ##4 ##5 ##6 {\handleMPsequence}%
   \else
     \PDFcode{\gMPa2 w}%
     \def\next##1 ##2 ##3 ##4 {\handleMPsequence}%
   \fi
   \let\handleMPsequence\dohandleMPsequence
   \resetMPstack
   \next}

%D The most complicated command is \type{concat}. \METAPOST\
%D applies this operator to \type{stroke}. At that moment the
%D points set by \type{curveto} and \type{moveto}, are already
%D fixed. In \PDF\ however the \type{cm} operator affects the
%D points as well as the pen (stroke). Like more \PDF\
%D operators, \type{cm} is defined in a bit ambiguous way.
%D The only save route for non||circular penshapes, is saving
%D the path, recalculating the points and applying the
%D transformation matrix in such a way that we can be sure
%D that its behavior is well defined. This comes down to
%D inverting the path and applying \type{cm} to that path as
%D well as the pen. This all means that we have to save the
%D path.

%D In \METAPOST\ there are three ways to handle a path $p$:
%D
%D \starttypen
%D draw p;  fill p;  filldraw p;
%D \stoptypen
%D
%D The last case outputs a \type{gsave fill grestore} before
%D \type{stroke}. Handling the path outside the main loops
%D saves about 40\% run time.\voetnoot{We can save some more by
%D following the \METAPOST\ output routine, but for the moment
%D we keep things simple.} Switching between the main loop and
%D the path loop is done by means of the recursely called
%D macro \type{\handleMPsequence}.

\def\handleMPpath%
  {\chardef\finiMPpath0
   \let\closeMPpath\relax
   \let\flushMPpath\flushnormalMPpath
   \resetMPstack
   \nofMPsegments1
   \let\handleMPsequence\dohandleMPpath
   \dohandleMPpath}

%D Most paths are drawn with simple round pens. Therefore we've
%D split up the routine in two.

\def\flushnormalMPsegment
  {\expandafter\ifcase\getMPkeyword{\the\nofMPsegments}\relax
     \PDFcode{\!MPgMPs1 \!MPgMPs2 l}%
   \or
     \PDFcode{\!MPgMPs1 \!MPgMPs2 \!MPgMPs3 \!MPgMPs4 \!MPgMPs5 \!MPgMPs6 c}%
   \or
     \PDFcode{\!MP\lastMPmoveX\space\!MP\lastMPmoveY\space l S}%
   \or
     \edef\lastMPmoveX{\gMPs1}% evt \!MP here
     \edef\lastMPmoveY{\gMPs2}%
     \PDFcode{\!MP\lastMPmoveX\space \!MP\lastMPmoveY\space m}%
   \fi}

\def\flushnormalMPpath%
  {\scratchcounter\nofMPsegments
   \nofMPsegments1
   \loop
     \flushnormalMPsegment
     \advance\nofMPsegments 1
     \ifnum\nofMPsegments<\scratchcounter
   \repeat}

\def\flushconcatMPsegment
  {\expandafter\ifcase\getMPkeyword{\the\nofMPsegments}\relax
     \doMPconcat{\gMPs1}\a{\gMPs2}\b%
     \PDFcode{\!MP\a\space\!MP\b\space l}%
   \or
     \doMPconcat{\gMPs1}\a{\gMPs2}\b%
     \doMPconcat{\gMPs3}\c{\gMPs4}\d%
     \doMPconcat{\gMPs5}\e{\gMPs6}\f%
     \PDFcode{\!MP\a\space\!MP\b\space
              \!MP\c\space\!MP\d\space
              \!MP\e\space\!MP\f\space c}%
   \or
     \bgroup
     \noMPtranslate
     \doMPconcat\lastMPmoveX\a\lastMPmoveY\b%
     \PDFcode{\!MP\a\space\!MP\b\space l S}%
     \egroup
   \or
     \edef\lastMPmoveX{\gMPs1}%
     \edef\lastMPmoveY{\gMPs2}%
     \doMPconcat\lastMPmoveX\a\lastMPmoveY\b%
     \PDFcode{\!MP\a\space\!MP\b\space m}%
   \fi}

\def\flushconcatMPpath%
  {\scratchcounter\nofMPsegments
   \nofMPsegments1
   \loop
     \flushconcatMPsegment
     \advance\nofMPsegments 1
     \ifnum\nofMPsegments<\scratchcounter
   \repeat}

%D The transformation of the coordinates is handled by one of
%D the macros Tanmoy posted to the \PDFTEX\ mailing list.
%D I rewrote and optimized the original macro to suit the other
%D macros in this module.
%D
%D \starttypen
%D \doMPconcat {x position} \xresult {y position} \yresult
%D \stoptypen
%D
%D By setting the auxiliary \DIMENSIONS\ \type{\dimen0} upto
%D \type{\dimen10} only once per path, we save over 20\% run
%D time. Some more speed was gained by removing some parameter
%D passing. These macros can be optimized a bit more by using
%D more constants. There is however not much need for further
%D optimization because penshapes usually are round and
%D therefore need no transformation. Nevertheless we move the
%D factor to the outer level and use a bit different \type{pt}
%D removal macro. Although the values represent base points,
%D we converted them to pure points, simply because those can
%D be converted back.

\def\MPconcatfactor{256}

\def\doMPreducedimen#1
  {\count0=\MPconcatfactor
   \advance\dimen#1 \ifdim\dimen#1>\!!zeropoint .5\else -.5\fi\count0
   \divide\dimen#1 \count0\relax}

% too inaccurate (see old pragma logo) 
% 
% \def\doMPreducedimen#1
%   {\count0=\MPconcatfactor
%    \divide\dimen#1 \count0\relax}

\def\doMPexpanddimen#1
  {\multiply\dimen#1 \MPconcatfactor\relax}

\def\presetMPconcat%
  {\dimen 0=\gMPs1 pt \doMPreducedimen 0    % r_x
   \dimen 2=\gMPs2 pt \doMPreducedimen 2    % s_x
   \dimen 4=\gMPs3 pt \doMPreducedimen 4    % s_y
   \dimen 6=\gMPs4 pt \doMPreducedimen 6    % r_y
   \dimen 8=\gMPs5 pt \doMPreducedimen 8    % t_x
   \dimen10=\gMPs6 pt \doMPreducedimen10 }  % t_y

\def\presetMPscale%
  {\dimen 0=\gMPs1 pt \doMPreducedimen 0 
   \dimen 2=\!!zeropoint
   \dimen 4=\!!zeropoint
   \dimen 6=\gMPs2 pt \doMPreducedimen 6 
   \dimen 8=\!!zeropoint 
   \dimen10=\!!zeropoint}  

\def\noMPtranslate% use this one grouped
  {\dimen 8=\!!zeropoint                    % t_x
   \dimen10=\!!zeropoint}                   % t_y

%D \starttypen 
%D \def\doMPconcat#1#2#3#4%
%D   {\dimen12=#1 pt \doMPreducedimen12 % p_x
%D    \dimen14=#3 pt \doMPreducedimen14 % p_y
%D    %
%D    \dimen16  \dimen 0
%D    \multiply \dimen16  \dimen 6
%D    \dimen20  \dimen 2
%D    \multiply \dimen20  \dimen 4
%D    \advance  \dimen16 -\dimen20
%D    %
%D    \dimen18  \dimen12
%D    \multiply \dimen18  \dimen 6
%D    \dimen20  \dimen14
%D    \multiply \dimen20  \dimen 4
%D    \advance  \dimen18 -\dimen20
%D    \dimen20  \dimen 4
%D    \multiply \dimen20  \dimen10
%D    \advance  \dimen18  \dimen20
%D    \dimen20  \dimen 6
%D    \multiply \dimen20  \dimen 8
%D    \advance  \dimen18 -\dimen20
%D    %
%D    \multiply \dimen12 -\dimen 2
%D    \multiply \dimen14  \dimen 0
%D    \advance  \dimen12  \dimen14
%D    \dimen20  \dimen 2
%D    \multiply \dimen20  \dimen 8
%D    \advance  \dimen12  \dimen20
%D    \dimen20  \dimen 0
%D    \multiply \dimen20  \dimen10
%D    \advance  \dimen12 -\dimen20
%D    %
%D    \doMPreducedimen16
%D    \divide   \dimen18  \dimen16 \doMPexpanddimen18
%D    \divide   \dimen12  \dimen16 \doMPexpanddimen12
%D    %
%D    \edef#2{\withoutpt{\the\dimen18}}% % p_x^\prime
%D    \edef#4{\withoutpt{\the\dimen12}}} % p_y^\prime
%D \stoptypen 

%D The following optimization resulted from some tests by 
%D and email exchanges with Sanjoy Mahajan. 
%D
%D \starttypen 
%D \def\doMPconcat#1#2#3#4%
%D   {\dimen12=#1 pt \doMPreducedimen12 % p_x
%D    \dimen14=#3 pt \doMPreducedimen14 % p_y
%D    %
%D    \dimen16  \dimen 0
%D    \multiply \dimen16  \dimen 6
%D    \dimen20  \dimen 2
%D    \multiply \dimen20  \dimen 4
%D    \advance  \dimen16 -\dimen20
%D    %
%D    \dimen18  \dimen12
%D    \multiply \dimen18  \dimen 6
%D    \dimen20  \dimen14
%D    \multiply \dimen20  \dimen 4
%D    \advance  \dimen18 -\dimen20
%D    \dimen20  \dimen 4
%D    \multiply \dimen20  \dimen10
%D    \advance  \dimen18  \dimen20
%D    \dimen20  \dimen 6
%D    \multiply \dimen20  \dimen 8
%D    \advance  \dimen18 -\dimen20
%D    %
%D    \multiply \dimen12 -\dimen 2
%D    \multiply \dimen14  \dimen 0
%D    \advance  \dimen12  \dimen14
%D    \dimen20  \dimen 2
%D    \multiply \dimen20  \dimen 8
%D    \advance  \dimen12  \dimen20
%D    \dimen20  \dimen 0
%D    \multiply \dimen20  \dimen10
%D    \advance  \dimen12 -\dimen20
%D    %
%D   %\ifdim\dimen16>1pt % oeps, can be < 1pt too
%D    \ifdim\dimen16=1pt \else
%D      \ifdim\dimen16>\MPconcatfactor pt
%D        \doMPreducedimen16
%D        \divide \dimen18 \dimen16 \doMPexpanddimen18
%D        \divide \dimen12 \dimen16 \doMPexpanddimen12
%D      \else
%D        \divide \dimen18 \dimen16 \doMPexpanddimen18 \doMPexpanddimen18
%D        \divide \dimen12 \dimen16 \doMPexpanddimen12 \doMPexpanddimen12
%D      \fi
%D    \fi
%D    %
%D    \edef#2{\withoutpt{\the\dimen18}}% % p_x^\prime
%D    \edef#4{\withoutpt{\the\dimen12}}} % p_y^\prime
%D \stoptypen 
%D
%D But, this one is still too inaccurate, so we now have: 

% \def\doMPconcat#1#2#3#4%
%   {\dimen12=#1pt % p_x
%    \dimen14=#3pt % p_y
%    %
%    % we should test for >-1024 too, but for the moment take the gamble
%    \chardef\MPfactor1\ifdim\dimen12<1024pt \ifdim\dimen14<1024pt 6\fi\fi
%    %
%    \multiply\dimen12 \MPfactor
%    \multiply\dimen14 \MPfactor
%    %
%    \doMPreducedimen12
%    \doMPreducedimen14
%    %
%    \dimen16  \dimen 0
%    \multiply \dimen16  \dimen 6
%    \dimen20  \dimen 2
%    \multiply \dimen20  \dimen 4
%    \advance  \dimen16 -\dimen20
%    %
%    \dimen18  \dimen12
%    \multiply \dimen18  \dimen 6
%    \dimen20  \dimen14
%    \multiply \dimen20  \dimen 4
%    \advance  \dimen18 -\dimen20
%    \dimen20  \dimen 4
%    \multiply \dimen20  \dimen10
%    \advance  \dimen18  \dimen20
%    \dimen20  \dimen 6
%    \multiply \dimen20  \dimen 8
%    \advance  \dimen18 -\dimen20
%    %
%    \multiply \dimen12 -\dimen 2
%    \multiply \dimen14  \dimen 0
%    \advance  \dimen12  \dimen14
%    \dimen20  \dimen 2
%    \multiply \dimen20  \dimen 8
%    \advance  \dimen12  \dimen20
%    \dimen20  \dimen 0
%    \multiply \dimen20  \dimen10
%    \advance  \dimen12 -\dimen20
%    %
%    \ifdim\dimen16=1pt \else
%      \ifdim\dimen16>\MPconcatfactor pt
%        \doMPreducedimen16
%        \divide \dimen18 \dimen16 \doMPexpanddimen18
%        \divide \dimen12 \dimen16 \doMPexpanddimen12
%      \else
%        \divide \dimen18 \dimen16 \doMPexpanddimen18 \doMPexpanddimen18
%        \divide \dimen12 \dimen16 \doMPexpanddimen12 \doMPexpanddimen12
%      \fi
%    \fi
%    %
%    \divide\dimen18 \MPfactor
%    \divide\dimen12 \MPfactor
%    %
%    \edef#2{\withoutpt{\the\dimen18}}% % p_x^\prime
%    \edef#4{\withoutpt{\the\dimen12}}} % p_y^\prime

%D We cannot use \type {\beginETEX} here since in plain we 
%D get \type {\outer} problems, sigh.  

% \beginTEX 

\def\MPcriteriumA {512pt} % scale 
\def\MPcriteriumB   {2pt} % scale 

% \endTEX
%

% \ifx\MPcriteriumA\undefined
% 
%   \newdimen\MPcriteriumA \MPcriteriumA=512pt
%   \newdimen\MPcriteriumB \MPcriteriumB=  2pt
% 
% \fi

\def\doMPconcat#1#2#3#4%
  {\dimen12=#1pt % p_x
   \dimen14=#3pt % p_y
   %
   \chardef\MPfactor0
   \ifdim\dimen4<\MPcriteriumB\ifdim\dimen4>-\MPcriteriumB
     \ifdim\dimen6<\MPcriteriumB\ifdim\dimen6>-\MPcriteriumB
       \ifdim\dimen8<\MPcriteriumB\ifdim\dimen8>-\MPcriteriumB
         \ifdim\dimen10<\MPcriteriumB\ifdim\dimen10>-\MPcriteriumB
           \chardef\MPfactor1
         \fi\fi
       \fi\fi
     \fi\fi
   \fi\fi
   \ifcase\MPfactor0 
     \chardef\MPfactor1
     \ifdim\dimen12<\MPcriteriumA\ifdim\dimen12>-\MPcriteriumA
       \ifdim\dimen14<\MPcriteriumA\ifdim\dimen14>-\MPcriteriumA
         \chardef\MPfactor16
       \fi\fi
     \fi\fi
   \fi
   %
   \multiply\dimen12 \MPfactor
   \multiply\dimen14 \MPfactor
   %
   \doMPreducedimen12
   \doMPreducedimen14
   %
   \dimen16  \dimen 0
   \multiply \dimen16  \dimen 6
   \dimen20  \dimen 2
   \multiply \dimen20  \dimen 4
   \advance  \dimen16 -\dimen20
   %
   \dimen18  \dimen12
   \multiply \dimen18  \dimen 6
   \dimen20  \dimen14
   \multiply \dimen20  \dimen 4
   \advance  \dimen18 -\dimen20
   \dimen20  \dimen 4
   \multiply \dimen20  \dimen10
   \advance  \dimen18  \dimen20
   \dimen20  \dimen 6
   \multiply \dimen20  \dimen 8
   \advance  \dimen18 -\dimen20
   %
   \multiply \dimen12 -\dimen 2
   \multiply \dimen14  \dimen 0
   \advance  \dimen12  \dimen14
   \dimen20  \dimen 2
   \multiply \dimen20  \dimen 8
   \advance  \dimen12  \dimen20
   \dimen20  \dimen 0
   \multiply \dimen20  \dimen10
   \advance  \dimen12 -\dimen20
   %
   \ifdim\dimen16=1pt \else
     \ifdim\dimen16>\MPconcatfactor pt
       \doMPreducedimen16
       \divide \dimen18 \dimen16 \doMPexpanddimen18
       \divide \dimen12 \dimen16 \doMPexpanddimen12
     \else
       \divide \dimen18 \dimen16 \doMPexpanddimen18 \doMPexpanddimen18
       \divide \dimen12 \dimen16 \doMPexpanddimen12 \doMPexpanddimen12
     \fi
   \fi
   %
   \divide\dimen18 \MPfactor
   \divide\dimen12 \MPfactor
   %
   \edef#2{\withoutpt{\the\dimen18}}% % p_x^\prime
   \edef#4{\withoutpt{\the\dimen12}}} % p_y^\prime
 
%D The following explanation of the conversion process was
%D posted to the \PDFTEX\ mailing list by Tanmoy. The original
%D macro was part of a set of macro's that included sinus and
%D cosinus calculations as well as scaling and translating. The
%D \METAPOST\ to \PDF\ conversion however only needs
%D transformation.

%M \start \switchnaarkorps [ss]

%D Given a point $(U_x, U_y)$ in user coordinates, the business
%D of \POSTSCRIPT\ is to convert it to device space. Let us say
%D that the device space coordinates are $(D_x, D_y)$. Then, in
%D \POSTSCRIPT\ $(D_x, D_y)$ can be written in terms of
%D $(U_x, U_y)$ in matrix notation, either as
%D
%D \plaatsformule
%D   \startformule
%D   \pmatrix{D_x&D_y&1\cr} = \pmatrix{U_x&U_y&1\cr}
%D                            \pmatrix{s_x&r_x&0\cr
%D                                     r_y&s_y&0\cr
%D                                     t_x&t_y&1\cr}
%D   \stopformule
%D
%D or
%D
%D \plaatsformule
%D   \startformule
%D    \pmatrix{D_x\cr D_y\cr 1} = \pmatrix{s_x&r_y&t_x\cr
%D                                         r_x&s_y&t_y\cr
%D                                         0  &0  &1  \cr}
%D                                \pmatrix{U_x\cr
%D                                         U_y\cr
%D                                         1  \cr}
%D   \stopformule
%D
%D both of which is a shorthand for the same set of equations:
%D
%D \plaatsformule
%D   \startformule
%D      D_x = s_x U_x + r_y U_y + t_x
%D   \stopformule
%D
%D \plaatsformule
%D   \startformule
%D      D_y = r_x U_x + s_y U_y + t_y
%D   \stopformule
%D
%D which define what is called an `affine transformation'.
%D
%D \POSTSCRIPT\ represents the `transformation matrix' as a
%D six element matrix instead of a $3\times 3$ array because
%D three of the elements are always~0, 0 and~1. Thus the above
%D transformation is written in postscript as $[s_x\, r_x\,
%D r_y\, s_y\, t_x\, t_y]$. However, when doing any
%D calculations, it is useful to go back to the original
%D matrix notation (whichever: I will use the second) and
%D continue from there.
%D
%D As an example, if the current transformation matrix is
%D $[s_x\, r_x\, r_y\, s_y\, t_x\, t_y]$ and you say \typ{[a b
%D c d e f] concat}, this means:
%D
%D \startsmaller
%D Take the user space coordinates and transform them to an
%D intermediate set of coordinates using array $[a\, b\, c\, d\,
%D e\, f]$ as the transformation matrix.
%D
%D Take the intermediate set of coordinates and change them to
%D device coordinates using array $[s_x\, r_x\, r_y\, s_y\, t_x\, t_y]$
%D as the transformation matrix.
%D \stopsmaller
%D
%D Well, what is the net effect? In matrix notation, it is
%D
%D \plaatsformule
%D   \startformule
%D     \pmatrix{I_x\cr I_y\cr 1\cr} = \pmatrix{a&c&e\cr
%D                                             b&d&f\cr
%D                                             0&0&1\cr}
%D                                    \pmatrix{U_x\cr
%D                                             U_y\cr
%D                                             1  \cr}
%D   \stopformule
%D
%D \plaatsformule
%D   \startformule
%D     \pmatrix{D_y\cr D_y\cr 1\cr} = \pmatrix{s_x&r_y&t_x\cr
%D                                             r_x&s_y&t_y\cr
%D                                             0  &0  &1  \cr}
%D                                    \pmatrix{I_x\cr
%D                                             I_y\cr
%D                                             1  \cr}
%D   \stopformule
%D
%D where $(I_x, I_y)$ is the intermediate coordinate.
%D
%D Now, the beauty of the matrix notation is that when there is
%D a chain of such matrix equations, one can always compose
%D them into one matrix equation using the standard matrix
%D composition law. The composite matrix from two matrices can
%D be derived very easily: the element in the $i$\hoog{th}
%D horizontal row and $j$\hoog{th} vertical column is
%D calculated by`multiplying' the $i$\hoog{th} row of the first
%D matrix and the $j$\hoog{th} column of the second matrix (and
%D summing over the elements). Thus, in the above:
%D
%D \plaatsformule
%D   \startformule
%D   \pmatrix{D_x\cr D_y\cr 1} = \pmatrix{s_x^\prime&r_y^\prime&t_x^\prime\cr
%D                                        r_x^\prime&s_y^\prime&t_y^\prime\cr
%D                                        0         &0         &0        \cr}
%D                               \pmatrix{U_x\cr
%D                                        U_y\cr
%D                                        1  \cr}
%D   \stopformule
%D
%D with
%D
%D \plaatsformule
%D   \startformule
%D      \eqalign
%D        {s_x^\prime & = s_x a + r_y b       \cr
%D         r_x^\prime & = r_x a + s_y b       \cr
%D         r_y^\prime & = s_x c + r_y d       \cr
%D         s_y^\prime & = r_x c + s_y d       \cr
%D         t_x^\prime & = s_x e + r_y f + t_x \cr
%D         t_y^\prime & = r_x e + s_y f + t_y \cr}
%D   \stopformule

%D In fact, the same rule is true not only when one is going
%D from user coordinates to device coordinates, but whenever
%D one is composing two `transformations' together
%D (transformations are `associative'). Note that the formula
%D is not symmetric: you have to keep track of which
%D transformation existed before (i.e.\ the equivalent of
%D $[s_x\, r_x\, r_y\, s_y\, t_x\, t_y]$) and which was
%D specified later (i.e.\ the equivalent of $[a\, b\, c\, d\,
%D e\, f]$). Note also that the language can be rather
%D confusing: the one specified later `acts earlier',
%D converting the user space coordinates to intermediate
%D coordinates, which are then acted upon by the pre||existing
%D transformation. The important point is that order of
%D transformation matrices cannot be flipped (transformations
%D are not `commutative').
%D
%D Now what does it mean to move a transformation matrix
%D before a drawing? What it means is that given a point
%D $(P_x, P_y)$ we need a different set of coordinates
%D $(P_x^\prime, P_y^\prime)$ such that if the transformation
%D acts on $(P_x^\prime, P_y^\prime)$, they produce $(P_x,
%D P_y)$. That is we need to solve the set of equations:
%D
%D \plaatsformule
%D   \startformule
%D     \pmatrix{P_x\cr P_y\cr 1\cr} = \pmatrix{s_x&r_y&t_x\cr
%D                                             r_x&s_y&t_y\cr
%D                                             0  &0  &1  \cr}
%D                                    \pmatrix{P_x^\prime\cr
%D                                             P_y^\prime\cr
%D                                             1         \cr}
%D   \stopformule
%D
%D Again matrix notation comes in handy (i.e. someone has
%D already solved the problem for us): we need the inverse
%D transformation matrix. The inverse transformation matrix can
%D be calculated very easily: 
%D
%D \plaatsformule
%D   \startformule
%D     \pmatrix{P_x^\prime\cr P_y^\prime\cr 1\cr} =
%D        \pmatrix{s_x^\prime&r_y^\prime&t_x^\prime\cr
%D                 r_x^\prime&s_y^\prime&t_y^\prime\cr
%D                 0  &0  &1  \cr}
%D        \pmatrix{P_x\cr
%D                 P_y\cr
%D                 1         \cr}
%D   \stopformule
%D
%D where, the inverse transformation matrix is given by
%D
%D \plaatsformule
%D   \startformule
%D     \eqalign
%D       {D          & = s_x s_y - r_x r_y           \cr
%D        s_x^\prime & = s_y / D                     \cr
%D        s_y^\prime & = s_x / D                     \cr
%D        r_x^\prime & = - r_x / D                   \cr
%D        r_y^\prime & = - r_y / D                   \cr
%D        t_x^\prime & = ( - s_y t_x + r_y t_y ) / D \cr
%D        t_y^\prime & = (   r_x t_x - s_x t_y ) / D \cr}
%D   \stopformule
%D
%D And you can see that when expanded out, this does
%D give the formulas:
%D
%D \plaatsformule
%D   \startformule
%D     P_x^\prime = { { s_y(p_x-t_x) + r_y(t_y-p_y) } \over
%D                    { s_x s_y-r_x r_y } }
%D   \stopformule
%D
%D \plaatsformule
%D   \startformule
%D     P_y^\prime = { { s_x(p_y-t_y) + r_x(t_x-p_x) } \over
%D                    { s_x*s_y-r_x*r_y } }
%D   \stopformule
%D
%D The code works by representing a real number by converting
%D it to a dimension to be put into a \DIMENSION\ register: 2.3 would
%D be represented as 2.3pt for example. In this scheme,
%D multiplying two numbers involves multiplying the \DIMENSION\
%D registers and dividing by 65536. Accuracy demands that the
%D division be done as late as possible, but overflow
%D considerations need early division.
%D
%D Division involves dividing the two \DIMENSION\ registers and
%D multiplying the result by 65536. Again, accuracy would
%D demand that the numerator be multiplied (and|/|or the
%D denominator divided) early: but that can lead to overflow
%D which needs to be avoided.
%D
%D If nothing is known about the numbers to start with (in
%D concat), I have chosen to divide the 65536 as a 256 in each
%D operand. However, in the series calculating the sine and
%D cosine, I know that the terms are small (because I never
%D have an angle greater than 45 degrees), so I chose to
%D apportion the factor in a different way.

%M \stop

%D The path is output using the values saved on the stack. If
%D needed, all coordinates are recalculated.

\def\finishMPpath%
  {\PDFcode{\ifcase\finiMPpath W n\or S\or f\or B\fi}}

\def\processMPpath%
  {\checkMPpath
   \ifcase\nofMPsegments\else
     \flushMPpath
     \closeMPpath
     \finishMPpath
   \fi 
   \let\handleMPsequence\dohandleMPsequence
   \resetMPstack
   \nofMPsegments0
   \handleMPsequence}

%D The following \METAPOST\ code is quite valid but, when
%D processed and converted to \PDF, will make a file
%D unprintable on a Hewlett Packard printer (from Acrobat
%D $v<=5$). Who is to blame, the driver of the OS layer in
%D between, is hard to determine, so we add an additional
%D check. 
%D 
%D \starttypen
%D clip currentpicture to origin -- cycle ; 
%D setbounds currentpicture to fullsquare scaled 5cm ; 
%D \stoptypen

\def\checkMPpath
  {\ifcase\finiMPpath       
     \ifnum\nofMPsegments<3 % n is one ahead
       \message{omitting zero clip path}%
       \nofMPsegments0 
     \fi 
   \fi}

%D In \PDF\ the \type{cm} operator must precede the path
%D specification. We therefore can output the \type{cm} at
%D the moment we encounter it.

\def\handleMPpathconcat%
  {\presetMPconcat
   \PDFcode{\gMPs1 \gMPs2 \gMPs3 \gMPs4 \gMPs5 \gMPs6 cm}%
   \resetMPstack}

\def\handleMPpathscale%
  {\presetMPscale
   \PDFcode{\gMPs1 0 0 \gMPs2 0 0 cm}%
   \resetMPstack}

%D This macro interprets the path and saves it as compact as
%D possible.

\def\dohandleMPpath#1%
  {\ifcase\lccode`#1\relax
     \@EA\dohandleMPpathA
   \else
     \@EA\dohandleMPpathB
   \fi#1}

%\def\dohandleMPpathA#1 %
%  {\setMPargument{#1}%
%   \handleMPsequence}

\let\dohandleMPpathA\setMPsequence

\def\dohandleMPpathB#1 %
  {\def\somestring{#1}%
   \ifx\somestring\PSlineto
     \setMPkeyword0
   \else\ifx\somestring\PScurveto
     \setMPkeyword1
   \else\ifx\somestring\PSrlineto
     \setMPkeyword2
   \else\ifx\somestring\PSmoveto
     \setMPkeyword3
   \else\ifx\somestring\PSclip
   % \chardef\finiMPpath0 % already 
     \let\handleMPsequence\processMPpath
   \else\ifx\somestring\PSgsave
     \chardef\finiMPpath3
   \else\ifx\somestring\PSgrestore
   \else\ifx\somestring\PSfill
     \ifcase\finiMPpath
       \chardef\finiMPpath2
       \let\handleMPsequence\processMPpath
     \fi
   \else\ifx\somestring\PSstroke
     \ifcase\finiMPpath
       \chardef\finiMPpath1
     \fi
     \let\handleMPsequence\processMPpath
   \else\ifx\somestring\PSclosepath
     \def\closeMPpath{\PDFcode{h}}%
   \else\ifx\somestring\PSconcat
     \let\flushMPpath\flushconcatMPpath
     \handleMPpathconcat
   \else\ifx\somestring\PSscale
     \let\flushMPpath\flushconcatMPpath
     \handleMPpathscale
   \fi\fi\fi\fi\fi\fi\fi\fi\fi\fi\fi\fi
   \handleMPsequence}

%D The main conversion command is:
%D
%D \starttypen
%D \convertMPtoPDF {filename} {x scale} {y scale}
%D \stoptypen
%D
%D The dimensions are derived from the bounding box. So we
%D only have to say:
%D
%D \starttypen
%D \convertMPtoPDF{mp-pra-1.eps}{1}{1}
%D \convertMPtoPDF{mp-pra-1.eps}{.5}{.5}
%D \stoptypen

%D \macros 
%D   {makeMPintoPDFobject,lastPDFMPobject}
%D
%D For experts there are a few more options. When attributes
%D are to be added, the code must be embedded in an object 
%D accompanied with the appropriate directives. One can 
%D influence this process with \type {\makeMPintoPDFobject}.
%D
%D This option defaults to~0, because \CONTEXT\ takes care 
%D of objects at another level, which saves some bytes.  
%D
%D \starttabulatie[|l|l|p|]
%D \NC 0 \NC never    \NC don't use an object    \NC\NR
%D \NC 1 \NC always   \NC always use an object   \NC\NR
%D \NC 2 \NC optional \NC use object when needed \NC\NR
%D \stoptabulatie 
%D 
%D The last object number used is avaliable in the macro 
%D \type {\lastPDFMPobject}.

\chardef\makeMPintoPDFobject=0 \def\lastPDFMPobject{0}

%D The additional code needed can be made available in the 
%D (global) macro \type {\currentPDFresources}.

\let\currentPDFresources\empty  

\newtoks\everyMPtoPDFconversion

\def\convertMPtoPDF#1#2#3%
  {\bgroup
   \ifx\pdfdecimaldigits\undefined\else \pdfdecimaldigits=5 \fi % new 
   \setbox\scratchbox\vbox\bgroup
     \forgetall
     \offinterlineskip
     \startMPresources
     \doprocessMPtoPDFfile{#1}{#2}{#3}} % {#1}{0#2}{0#3} would be saver 

\def\processMPtoPDFfile% file xscale yscale 
  {\bgroup
   \let\finishMPgraphic\egroup
   \doprocessMPtoPDFfile}

\def\doprocessMPtoPDFfile#1#2#3% file xscale yscale 
  {\setMPspecials
   \the\everyMPtoPDFconversion
   \catcode`\^^M=\@@endofline
   \startMPscanning
   \let\do\empty
   \xdef\MPxscale{#2}%
   \xdef\MPyscale{#3}%
   \donefalse
   \let\handleMPsequence\dohandleMPsequence
   \message{[MP to PDF]}% was: [MP to PDF #1] but there is a (#1) anyway 
   \input#1\relax}

% strange rounding/clip in pdftex/viewer
% 
% \def\finishMPgraphic
%   {\stopMPresources
%    \egroup
%    \ifx\pdftexversion\undefined\else\ifnum\pdftexversion<14 % for the moment 
%      \chardef\makeMPintoPDFobject=0 
%    \fi\fi
%    \ifcase\makeMPintoPDFobject\or\or\ifx\currentPDFresources\empty\else
%      \chardef\makeMPintoPDFobject=1 
%    \fi\fi
%    \setbox\scratchbox=\vbox
%      {\forgetall
%       \hbox
%         {\PDFcode{q \MPxscale\space 0 0 \MPyscale\space \MPxoffset\space \MPyoffset\space cm}%
%          \lower\MPyshift\box\scratchbox % unscaled shift 
%          \PDFcode{Q}}}%
%    \ht\scratchbox\MPheight
%    \wd\scratchbox\MPwidth
%    \dp\scratchbox\!!zeropoint
%    \ifcase\makeMPintoPDFobject
%      \box\scratchbox
%    \or
%      \immediate\pdfxform resources{\currentPDFresources}\scratchbox
%      \xdef\lastPDFMPobject{\the\pdflastxform}%
%      \pdfrefxform\lastPDFMPobject
%      \global\let\currentPDFresources\empty
%    \else
%      \box\scratchbox
%    \fi
%    \egroup}
%
% funny clip in viewer
%
% \setbox\scratchbox=\vbox
%   {\forgetall
%    \dimen0=\MPllx bp
%    \dimen2=\MPlly bp
%    \setbox\scratchbox=\hbox{\hskip-\dimen0\raise-\dimen2\box\scratchbox}%
%    \ht\scratchbox=\!!zeropoint
%    \dp\scratchbox=\!!zeropoint
%    \wd\scratchbox=\!!zeropoint
%    \hbox
%      {\PDFcode{q \MPxscale\space 0 0 \MPyscale\space 0 0 cm}%
%       \lower\MPshift\box\scratchbox
%       \PDFcode{Q}}}%

% \let\PDFMPformoffset\!!zeropoint

\def\PDFMPformoffset
  {\ifx\objectoffset\undefined\!!zeropoint\else\objectoffset\fi}

\def\finishMPgraphic
  {\stopMPresources
   \egroup
   \ifx\pdftexversion\undefined\else\ifnum\pdftexversion<14 % for the moment 
     \chardef\makeMPintoPDFobject0 
   \fi\fi
   \ifcase\makeMPintoPDFobject\or\or\ifx\currentPDFresources\empty\else
     \chardef\makeMPintoPDFobject1 
   \fi\fi
   \setbox\scratchbox\vbox 
     {\forgetall
      \hbox 
        {\PDFcode{q \MPxscale\space 0 0 \MPyscale\space \MPxoffset\space \MPyoffset\space cm}%
         \lower\MPyshift\box\scratchbox % unscaled shift 
         \PDFcode{Q}}}%
   \ht\scratchbox\MPheight
   \wd\scratchbox\MPwidth
   \dp\scratchbox\!!zeropoint\relax
   \ifcase\makeMPintoPDFobject
     \box\scratchbox
   \or
     \scratchdimen\PDFMPformoffset\relax
     \ifdim\scratchdimen>\!!zeropoint % compensate for error 
       \setbox\scratchbox=\vbox spread 2\scratchdimen
         {\forgetall
          \vss
          \hbox spread 2\scratchdimen
            {\hss
             \box\scratchbox
             \hss}%
          \vss}%
     \fi
     \immediate\pdfxform resources{\currentPDFresources}\scratchbox
     \xdef\lastPDFMPobject{\the\pdflastxform}%
     \ifdim\scratchdimen>\!!zeropoint % compensate for error
       \vbox to \MPheight 
         {\forgetall
          \vss\hbox to \MPwidth{\hss\pdfrefxform\lastPDFMPobject\hss}\vss}%
     \else
       \pdfrefxform\lastPDFMPobject
     \fi
     \global\let\currentPDFresources\empty
   \else
     \box\scratchbox
   \fi
   \egroup
   \endinput}

%D \macros 
%D   {deleteMPgraphic,
%D    startMPresources,
%D    stopMPresources}
%D 
%D Here are a few hooks for \CONTEXT\ specific things. 

\ifx\deleteMPgraphic\undefined
  \def\deleteMPgraphic#1{}
\fi

\ifx\startMPresources\undefined
  \let\startMPresources\relax
  \let\stopMPresources\relax
\fi

%D \macros
%D   {twodigitMPoutput}
%D
%D We can limit the precision to two digits after the comma 
%D by saying: 
%D
%D \starttypen
%D \twodigitMPoutput
%D \stoptypen
%D
%D This option only works in \CONTEXT\ combined with \ETEX. 

\def\twodigitMPoutput%
  {\let\!MP        \twodigitrounding
   \def\!MPgMPs##1{\twodigitrounding{\gMPs##1}}%
   \def\!MPgMPa##1{\twodigitrounding{\gMPa##1}}}

\let\!MP    \empty
\let\!MPgMPa\gMPa
\let\!MPgMPs\gMPs

%D This kind of conversion is possible because \METAPOST\
%D does all the calculations. Converting other \POSTSCRIPT\
%D files would drive both me and \TEX\ crazy.

\ifx\undefined\StopLatexHack \else \StopLatexHack \fi 

\protect \endinput
